# Supplementary material for: Bayesian Adaptive Selection of Basis Functions for Functional Data Representation
Source: arXiv:2204.03115 ancillary file (2022-05-26)
Supplement: Supplementary file 1 [file supplementary_material.pdf]

# Bayesian Adaptive Selection of Basis Functions for Functional Data Representation

# Supplementary Material

Pedro Henrique T. O. Sousa[1]*, Camila P. E. de Souza[2], Ronaldo Dias[1]

[1]Department of Statistics, University of Campinas, SP, Brazil
[2]Department of Statistical and Actuarial Sciences, University of Western Ontario, ON, Canada
*Correspondence: phtos_est@gmail.com

## 1 Synthetic data studies MSEs

Table 1: MSEs of the OLS methods and the proposed Bayesian models according to the different configurations tested with the B-spline bases (1st study with synthetic data).

| $\sigma$ | K | $\mu$ (Hyperparameter) | | | | | | | | | $\mu$ (Parameter) | OLS |
|---|---|---|---|---|---|---|---|---|---|---|---|---|
| | | 0.1 | 0.2 | 0.3 | 0.4 | 0.5 | 0.6 | 0.7 | 0.8 | 0.9 | | |
| 0.1 | 5 | 7.70E-03 | 7.64E-03 | 7.65E-03 | 7.59E-03 | 7.68E-03 | 7.62E-03 | 7.71E-03 | 7.68E-03 | 7.47E-03 | 7.65E-03 | 7.23E-03 |
| | 6 | 1.02E-02 | 1.02E-02 | 1.03E-02 | 1.02E-02 | 1.03E-02 | 1.04E-02 | 1.03E-02 | 1.02E-02 | 1.02E-02 | 1.02E-02 | 1.03E-02 |
| | 7 | 2.36E-03 | 2.43E-03 | 2.19E-03 | 2.21E-03 | 2.15E-03 | 2.16E-03 | 2.13E-03 | 2.16E-03 | 2.21E-03 | 2.38E-03 | 2.13E-03 |
| | 8 | 5.11E-03 | 4.72E-03 | 4.62E-03 | 4.70E-03 | 4.56E-03 | 4.60E-03 | 4.28E-03 | 4.21E-03 | 4.14E-03 | 5.20E-03 | 4.11E-03 |
| | 9 | 2.34E-03 | 1.96E-03 | 1.69E-03 | 1.32E-03 | 1.34E-03 | 1.12E-03 | 1.10E-03 | 1.06E-03 | 1.03E-03 | 2.27E-03 | 9.43E-04 |
| | 10 | 7.14E-05 | 8.05E-05 | 2.78E-05 | 1.13E-04 | 6.26E-05 | 1.15E-04 | 1.43E-04 | 1.67E-04 | 1.48E-04 | 9.17E-05 | 1.16E-04 |
| | 11 | 7.65E-04 | 4.87E-04 | 4.59E-04 | 4.47E-04 | 5.25E-04 | 4.48E-04 | 4.91E-04 | 3.84E-04 | 4.41E-04 | 7.18E-04 | 3.31E-04 |
| | 12 | 7.36E-04 | 6.88E-04 | 5.37E-04 | 6.24E-04 | 5.21E-04 | 6.23E-04 | 5.75E-04 | 4.84E-04 | 4.22E-04 | 7.84E-04 | 4.00E-04 |
| | 13 | 1.66E-04 | 3.01E-04 | 2.81E-04 | 2.54E-04 | 2.29E-04 | 2.95E-04 | 3.86E-04 | 3.57E-04 | 3.57E-04 | 3.27E-04 | 2.84E-04 |
| | 14 | 4.69E-04 | 5.09E-04 | 4.03E-04 | 4.21E-04 | 4.04E-04 | 3.30E-04 | 2.99E-04 | 2.70E-04 | 3.62E-04 | 5.17E-04 | 2.72E-04 |
| | 15 | 4.75E-04 | 3.41E-04 | 3.58E-04 | 4.08E-04 | 2.06E-04 | 4.05E-04 | 2.99E-04 | 2.60E-04 | 3.98E-04 | 5.26E-04 | 3.12E-04 |
| | 20 | 1.28E-03 | 8.21E-04 | 8.59E-04 | 9.52E-04 | 4.50E-04 | 4.70E-04 | 5.02E-04 | 5.09E-04 | 4.39E-04 | 1.41E-03 | 4.30E-04 |
| | 25 | 1.57E-03 | 1.06E-03 | 9.17E-04 | 7.63E-04 | 6.06E-04 | 6.93E-04 | 7.55E-04 | 6.64E-04 | 7.94E-04 | 1.56E-03 | 6.00E-04 |
| | 30 | 3.57E-03 | 1.75E-03 | 1.00E-03 | 1.12E-03 | 9.45E-04 | 7.78E-04 | 7.92E-04 | 9.64E-04 | 9.08E-04 | 4.22E-03 | 7.59E-04 |
| 0.5 | 5 | 1.87E-02 | 1.91E-02 | 2.05E-02 | 2.04E-02 | 1.59E-02 | 1.07E-02 | 1.13E-02 | 1.15E-02 | 8.22E-03 | 1.93E-02 | 8.59E-03 |
| | 6 | 2.84E-02 | 2.10E-02 | 1.64E-02 | 1.32E-02 | 1.27E-02 | 1.11E-02 | 1.17E-02 | 1.20E-02 | 1.19E-02 | 2.21E-02 | 1.30E-02 |
| | 7 | 1.07E-02 | 1.25E-02 | 7.73E-03 | 4.88E-03 | 3.70E-03 | 5.96E-03 | 4.76E-03 | 5.11E-03 | 3.69E-03 | 1.08E-02 | 4.32E-03 |
| | 8 | 1.35E-02 | 1.44E-02 | 1.11E-02 | 1.10E-02 | 1.23E-02 | 1.09E-02 | 7.02E-03 | 8.02E-03 | 6.22E-03 | 1.58E-02 | 6.78E-03 |
| | 9 | 1.86E-02 | 1.43E-02 | 9.70E-03 | 6.01E-03 | 6.30E-03 | 3.32E-03 | 4.54E-03 | 5.15E-03 | 4.53E-03 | 1.95E-02 | 4.05E-03 |
| | 10 | 4.00E-03 | 7.59E-03 | 7.15E-03 | 7.92E-03 | 6.44E-03 | 5.17E-03 | 3.37E-03 | 2.17E-03 | 3.72E-03 | 4.72E-03 | 2.89E-03 |
| | 11 | 9.88E-03 | 8.19E-03 | 5.24E-03 | 7.02E-03 | 7.06E-03 | 6.71E-03 | 8.25E-03 | 3.06E-03 | 4.57E-03 | 9.20E-03 | 4.57E-03 |
| | 12 | 2.24E-02 | 2.20E-02 | 1.61E-02 | 1.64E-02 | 1.63E-02 | 1.52E-02 | 9.77E-03 | 7.17E-03 | 4.75E-03 | 2.29E-02 | 7.09E-03 |
| | 13 | 2.55E-02 | 1.66E-02 | 1.62E-02 | 1.59E-02 | 1.56E-02 | 1.25E-02 | 9.99E-03 | 4.98E-03 | 7.00E-03 | 2.66E-02 | 6.34E-03 |
| | 14 | 2.41E-02 | 2.39E-02 | 2.11E-02 | 2.02E-02 | 1.37E-02 | 1.37E-02 | 8.66E-03 | 4.96E-03 | 8.20E-03 | 2.26E-02 | 6.48E-03 |
| | 15 | 2.87E-02 | 2.43E-02 | 2.19E-02 | 1.91E-02 | 1.53E-02 | 1.03E-02 | 7.16E-03 | 5.32E-03 | 6.23E-03 | 2.91E-02 | 7.68E-03 |
| | 20 | 5.19E-02 | 4.07E-02 | 2.72E-02 | 2.38E-02 | 1.81E-02 | 1.24E-02 | 8.54E-03 | 8.05E-03 | 7.39E-03 | 4.52E-02 | 1.07E-02 |
| | 25 | 7.01E-02 | 3.03E-02 | 2.12E-02 | 1.44E-02 | 1.08E-02 | 1.06E-02 | 8.51E-03 | 1.16E-02 | 1.20E-02 | 7.61E-02 | 1.50E-02 |
| | 30 | 7.87E-02 | 5.22E-02 | 3.98E-02 | 3.44E-02 | 2.29E-02 | 1.34E-02 | 1.21E-02 | 1.26E-02 | 1.32E-02 | 8.19E-02 | 1.90E-02 |

Table 2: MSEs of the OLS methods and the proposed Bayesian models according to the different configurations tested with the B-spline bases (2nd study with synthetic data).

| $\sigma$ | K | $\mu$ (Hyperparameter) | | | | | | | | | $\mu$ (Parameter) | OLS |
|---|---|---|---|---|---|---|---|---|---|---|---|---|
| | | 0.1 | 0.2 | 0.3 | 0.4 | 0.5 | 0.6 | 0.7 | 0.8 | 0.9 | | |
| 0.1 | 5 | 3.70E-01 | 3.70E-01 | 3.71E-01 | 3.70E-01 | 3.74E-01 | 3.67E-01 | 3.70E-01 | 3.63E-01 | 3.61E-01 | 3.70E-01 | 3.58E-01 |
| | 10 | 3.81E-04 | 4.04E-04 | 3.95E-04 | 4.70E-04 | 3.70E-04 | 4.60E-04 | 3.73E-04 | 4.29E-04 | 4.06E-04 | 4.05E-04 | 4.00E-04 |
| | 15 | 4.90E-04 | 4.73E-04 | 4.39E-04 | 3.11E-04 | 3.14E-04 | 4.18E-04 | 3.60E-04 | 2.71E-04 | 2.94E-04 | 5.37E-04 | 3.08E-04 |
| | 20 | 1.27E-03 | 1.29E-03 | 1.19E-03 | 1.15E-03 | 1.03E-03 | 7.54E-04 | 7.52E-04 | 5.68E-04 | 4.06E-04 | 1.30E-03 | 4.29E-04 |
| | 25 | 1.39E-03 | 1.19E-03 | 9.21E-04 | 7.49E-04 | 7.51E-04 | 6.99E-04 | 6.93E-04 | 6.19E-04 | 5.79E-04 | 1.34E-03 | 5.99E-04 |
| | 30 | 1.57E-03 | 1.67E-03 | 1.28E-03 | 1.40E-03 | 1.15E-03 | 1.21E-03 | 1.31E-03 | 9.60E-04 | 8.03E-04 | 1.70E-03 | 7.58E-04 |
| 0.5 | 5 | 3.80E-01 | 3.80E-01 | 3.74E-01 | 3.74E-01 | 3.75E-01 | 3.77E-01 | 3.76E-01 | 3.69E-01 | 3.69E-01 | 3.92E-01 | 3.60E-01 |
| | 10 | 2.36E-02 | 1.99E-02 | 1.59E-02 | 9.57E-03 | 6.32E-03 | 7.31E-03 | 1.19E-02 | 7.96E-03 | 4.30E-03 | 2.30E-02 | 3.18E-03 |
| | 15 | 3.44E-02 | 2.10E-02 | 1.25E-02 | 9.72E-03 | 7.23E-03 | 7.14E-03 | 5.51E-03 | 6.12E-03 | 5.94E-03 | 3.67E-02 | 7.66E-03 |
| | 20 | 5.39E-02 | 3.40E-02 | 2.28E-02 | 2.03E-02 | 1.06E-02 | 8.27E-03 | 9.00E-03 | 1.05E-02 | 8.44E-03 | 5.04E-02 | 1.07E-02 |
| | 25 | 5.37E-02 | 4.93E-02 | 1.99E-02 | 1.56E-02 | 1.47E-02 | 1.14E-02 | 1.40E-02 | 1.60E-02 | 9.78E-03 | 6.94E-02 | 1.50E-02 |
| | 30 | 7.20E-02 | 4.40E-02 | 3.32E-02 | 1.79E-02 | 1.41E-02 | 1.65E-02 | 1.84E-02 | 1.58E-02 | 1.67E-02 | 8.34E-02 | 1.90E-02 |

Table 3: MSEs of the OLS methods and the proposed Bayesian models according to the different configurations tested with the Fourier bases (2nd study with synthetic data).

| $\mu$ (Hyperparameter) | $\sigma$ | |
|---|---|---|
| | 0.1 | 0.5 |
| 0.01 | 1.92E-05 | 4.74E-04 |
| 0.02 | 6.25E-06 | 1.87E-03 |
| 0.03 | 6.12E-06 | 1.45E-03 |
| 0.04 | 1.90E-05 | 1.58E-03 |
| 0.05 | 3.69E-05 | 1.82E-03 |
| 0.06 | 3.31E-05 | 1.86E-03 |
| 0.07 | 3.21E-05 | 1.55E-03 |
| 0.08 | 2.75E-05 | 1.83E-03 |
| 0.09 | 2.78E-05 | 1.77E-03 |
| 0.1 | 8.26E-05 | 1.78E-03 |
| 0.2 | 5.79E-05 | 2.31E-03 |
| 0.3 | 7.35E-05 | 2.43E-03 |
| 0.4 | 8.55E-05 | 3.17E-03 |
| 0.5 | 7.25E-05 | 5.25E-03 |
| 0.6 | 1.32E-04 | 8.45E-03 |
| 0.7 | 1.23E-04 | 1.01E-02 |
| 0.8 | 2.36E-04 | 1.58E-02 |
| 0.9 | 3.69E-04 | 1.72E-02 |
| $\mu$ (Parameter) | 7.97E-05 | 1.84E-03 |
| OLS | 7.33E-04 | 1.83E-02 |

## 2 LASSO and Bayesian LASSO vs Proposed model

In addition to the smoothing and adaptive base selection method proposed herein, there are other methods which are also capable of inducing regularization and selection.

There are two methods in the statistical literature of linear regression which are widely known and have the properties highlighted here: the LASSO frequentist method (Least Ab-

solute Shrinkage and Selection Operator) presented by Tibshirani in 1996 and its Bayesian version, the Bayesian LASSO proposed by Park and Casella in 2008.

Through the frequentist approach, LASSO seeks to optimize the objective function:

$$\|\boldsymbol{y} - \boldsymbol{X}\boldsymbol{\beta}\|_2^2 + \lambda\|\boldsymbol{\beta}\|_1. \tag{1}$$

In which: $\boldsymbol{y}$ is already standardized so that it has a zero mean, $\boldsymbol{X}$ is the covariate matrix, $\boldsymbol{\beta}$ is the vector of coefficients to be estimated and $\lambda$ is the regularization parameter.

By the Bayesian approach, Bayesian LASSO obtains its estimates from samples of the following posterior distribution (Park and Casella, 2008):

$$\pi(\boldsymbol{\beta}, \sigma^2|\boldsymbol{y}) \propto \pi(\sigma^2)(\sigma^2)^{-\frac{(n+p-1)}{2}} \exp\left\{ -\frac{\|\boldsymbol{y} - \boldsymbol{X}\boldsymbol{\beta}\|_2^2}{2\sigma^2} - \lambda\sum_{j=1}^{p} \frac{|\beta_j|}{\sqrt{\sigma^2}} \right\}. \tag{2}$$

In which: $\lambda$ is a smoothing parameter that can be fixed as described in Expression (2), or it can be considered random in order to assign a prior to it.

Both techniques were presented and disseminated in the context of regression analysis, which is a similar field of study, but different from the area of functional data analysis. Therefore, such techniques can be used to adjust functional data by simply using the elements $B_k(.)'$s where covariates are normally used.

Thus, the objective of this section is to present a comparative analysis between the models mentioned here and the proposed model. To do so, two studies were carried out, the first using synthetic data and basis functions in accordance with what is described in subsection 3.3.1 in the main text, and the second uses a real database with several covariates.

## 2.1 Comparison with proposed model

As previously described, the synthetic data used in this study were generated in accordance with what is described in subsection 3.3.1 in the main text, meaning that the data generated here from a linear combination of B-splines, whose coefficient vector is $(-2, 0, 1.5, 1.5, 0, -1, -0.5, -1, 0, 0)$. As the objective here is to compare the performance of different models, it will be considered that $K = 10$, so that the bases used in the models are exactly the same bases used in the data generation.

As the purpose of this section is to compare the performance of the models and as the LASSO and Bayesian LASSO methods were not developed to simultaneously estimate several functionals, it was decided to use $m = 1$. Thus, in addition to greater computational feasibility, the comparison can be performed directly without the need (in the case of the adversary models) to establish a procedure that summarizes the results obtained for each functional.

In order for the comparison to be legitimate, each of the models was run 100 times with different observational data, meaning 100 replications of observational data were used.

We used the `blasso` function of the *monomvn* package (Gramacy, 2018) of the R statistical software program to obtain the Bayesian LASSO estimates, whose default considers a prior distribution in the regularization parameter $\lambda$. Therefore, a fair comparison can be made with the version of the proposed model, which also assigns a prior distribution for the $\mu$ component, which induces regularization and selection.

The mode (maximum a posteriori), the mean or the median can be used as a summary measure of the posterior samples. With this in mind, the performances in the Bayesian model replications were evaluated according to each of these summary measures.

Next, the boxplots of the performance metrics generated from applying the Bayesian LASSO model in the replications according to each summary measure are found in Appendix A. It is possible to notice that there is no significant difference between the results obtained by each metric. As the mode is the summary measure chosen to be used in the posterior samples generated by the proposed model, then it was decided to also use it in the posterior samples generated by Bayesian LASSO.

Although Park and Casella makes it clear that Bayesian LASSO matches LASSO when using the posterior mode and $\lambda$ is fixed, as in the default of the `blasso` function the regularization parameter has an associated prior, the results between them will naturally be different.

The `glmnet` function (Friedman et al., 2010) was used to obtain the LASSO estimates, which receives the same name as its source package and which is also available in the R software program.

In order to evaluate the proposed model performance, once we have $m = 1$ in this comparative study, the metric given by Eq. (16) in the main text takes the following form:

$$1 - \frac{(n_i - 1)(\boldsymbol{y_{i.}} - \boldsymbol{B}\,\mathrm{diag}(\hat{\boldsymbol{Z}}_{\boldsymbol{.i}})\hat{\boldsymbol{\beta}}_{\boldsymbol{.i}})'(\boldsymbol{y_{i.}} - \boldsymbol{B}\,\mathrm{diag}(\hat{\boldsymbol{Z}}_{\boldsymbol{.i}})\hat{\boldsymbol{\beta}}_{\boldsymbol{.i}})}{\left(n_i - \sum_{k=1}^{K} Z_{ki}\right)\left(\boldsymbol{y_{i.}} - \frac{1}{n_i}\sum_{j=1}^{n_i} y_{ij}\right)'\left(\boldsymbol{y_{i.}} - \frac{1}{n_i}\sum_{j=1}^{n_i} y_{ij}\right)}, \tag{3}$$

whereas it is necessary to modify the performance metric (3) slightly in order to evaluate the performance of LASSO and Bayesian LASSO in this comparative analysis so that one has:

$$1 - \frac{(n_i - 1)(\boldsymbol{y_{i.}} - \boldsymbol{B\beta})'(\boldsymbol{y_{i.}} - \boldsymbol{B\beta})}{\left(n_i - \sum_{k=1}^{K} I_{\{|\beta_k|>0\}}\right)\left(\boldsymbol{y_{i.}} - \frac{1}{n_i}\sum_{j=1}^{n_i} y_{ij}\right)'\left(\boldsymbol{y_{i.}} - \frac{1}{n_i}\sum_{j=1}^{n_i} y_{ij}\right)}. \tag{4}$$

In which: $\boldsymbol{\beta}$ is the vector of coefficients returned by LASSO (or Bayesian LASSO, if applicable).

Evidently the use of metric (4) is necessary for LASSO and Bayesian LASSO, as both models do not contain the latent variable vector $\boldsymbol{Z}$. So, for $m = 1$, as is the case with this application for comparison between models, the only difference between the metric (4) and the metric (16) is that in (4) only the vector of coefficients is used, instead of a vector whose components are characterized by the product of a given partial coefficient with the respective latent variable $Z_{ki}$.

Figure 1 presents the LASSO results for each tested $\lambda$ according to the data dispersion degree used.

As in the case of LASSO, you need to manually define the smoothing parameter $\lambda$, so a grid of values was defined for $\lambda$ characterized by a sequence that was generated in the R software program as follows: `seq(0.001,1,length=9)` for $\sigma = 0.1$ and `seq(0.001,5,length=9)` for $\sigma = 0.5$. Both sequences have the same length, but the second has values that extend up to 5, from which point it is already observed that the regularization becomes too intense. Thus, LASSO was run for each value of this sequence and for each of the 100 previously defined replications, and then the performance metric (4) was subsequently calculated.

A point which should be highlighted is that the `glmnet` function works in the optimization procedure of the following objective function:

$$\min_{(\beta_0,\boldsymbol{\beta})} \frac{1}{2n}\sum_{i=1}^{n}(y_i - \beta_0 - \boldsymbol{x_i'\beta})^2 + \lambda_{glmnet}\left[\frac{(1-a)}{2} \parallel \boldsymbol{\beta} \parallel_2^2 + a \parallel \boldsymbol{\beta} \parallel_2\right].$$

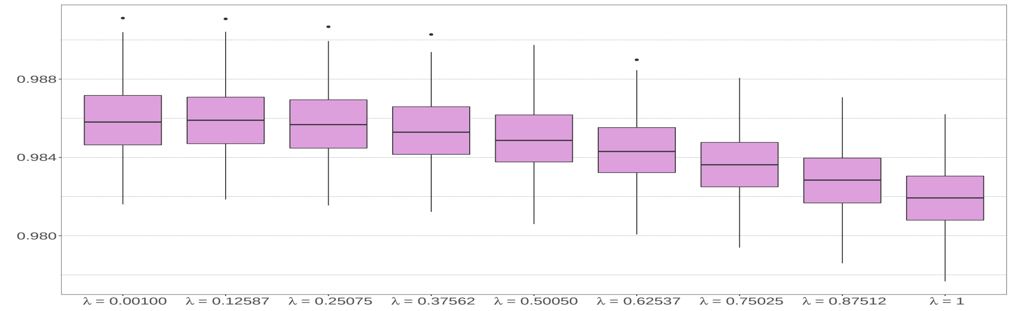


(a) Data with $\sigma = 0.1$.

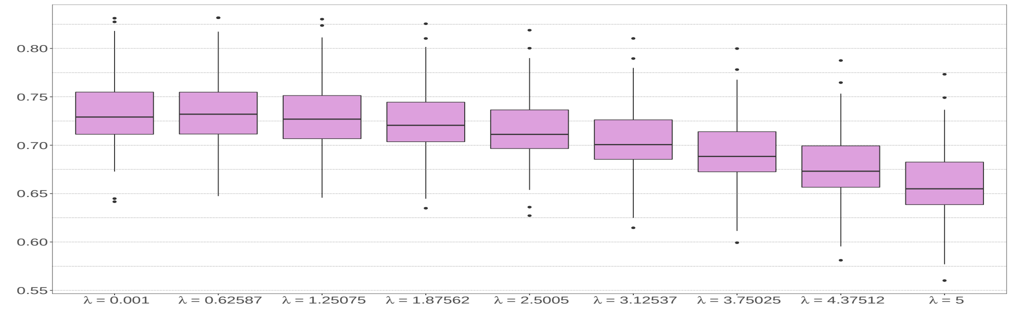


(b) Data with $\sigma = 0.5$.

Figure 1: Boxplots of the metric (4) for the various LASSO model configurations tested, according to the data dispersion degree.

In which: $\lambda_{glmnet} \geq 0$ is the regularization parameter used as input in the function and $0 \leq a \leq 1$. When $a = 0$, there is Ridge regression, and when $a = 1$, there is LASSO.

Thus, in order to apply LASSO in such a way that the regularization parameter complies with Expression (1), it is initially necessary to carry out a transformation in the regularization parameter that will be used in the function's input. Specifically for LASSO, there is $\lambda = 2n\lambda_{glmnet}$, and therefore $\lambda_{glmnet} = \frac{\lambda}{2n}$.

Figure 2 shows the model results for each $\mu$ according to the data dispersion degree used.

As the procedure to search for the smoothing element in a grid tends to provide better results than a procedure that automatically defines it, although it is computationally more costly, and as this manual procedure was used for LASSO, for fair comparison, a grid was defined ($\mu \in \{0.1,\ 0.2,\ 0.3,\ 0.4,\ 0.5,\ 0.6,\ 0.7,\ 0.8,\ 0.9\}$) of search for the best value of $\mu$, taking into account that the LASSO will be confronted with the version of the proposed model that considers $\mu$ as a hyperparameter.

It is not difficult to see that the proposed model has a low sensitivity in relation to the definition of the $\mu$ hyperparameter, but this ends up being a positive factor as it manages to smooth and select bases, providing good estimates, regardless of the a priori attributions. The same is not observed in LASSO, which returns worse fits as the regularization parameter $\lambda$ becomes too large. Another advantage over LASSO is the existence of a limited domain for $\mu$, while $\lambda$ can assume any non-negative value for the latter, making the search for the best difficult.

Figures 3 and 4 present the results considering both performance metrics: metric (16) and MSE, respectively.

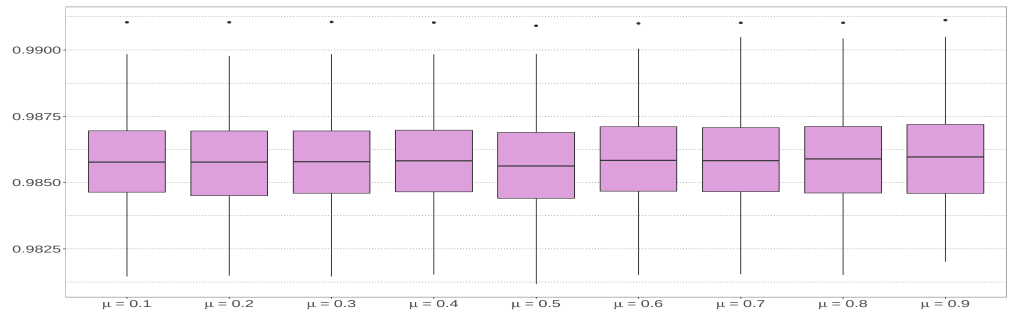


(a) Data with $\sigma = 0.1$.

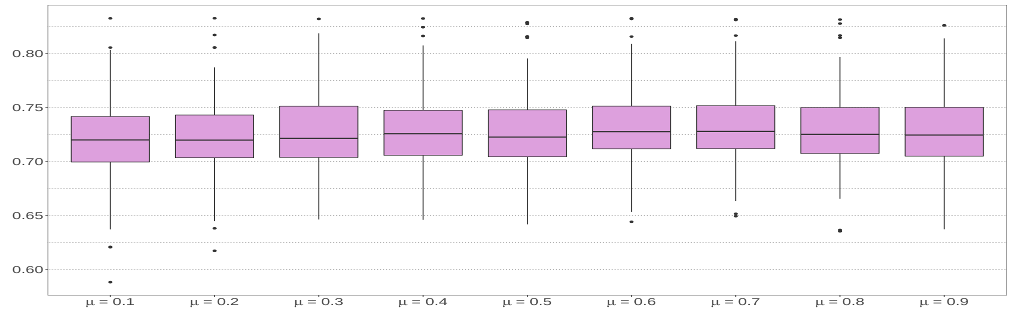


(b) Data with $\sigma = 0.5$.

Figure 2: Boxplots of the metric (16) for the different configurations of the proposed model with $\mu$ as the hyperparameter, according to the data dispersion degree.

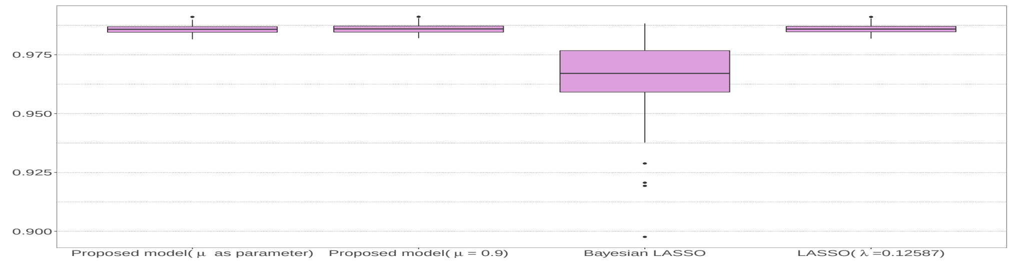


(a) Data with $\sigma = 0.1$.

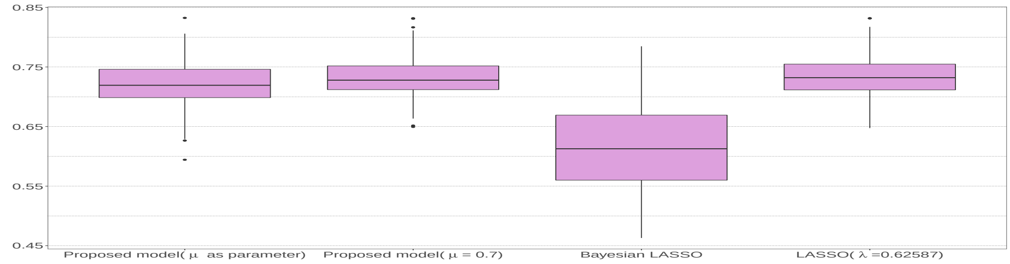


(b) Data with $\sigma = 0.5$.

Figure 3: Boxplots of the metric (16) (versions of the proposed model) and metric (4) (LASSO and Bayesian LASSO), according to the data dispersion degree.

In the case of LASSO, the average of the one hundred values returned by the perfor-

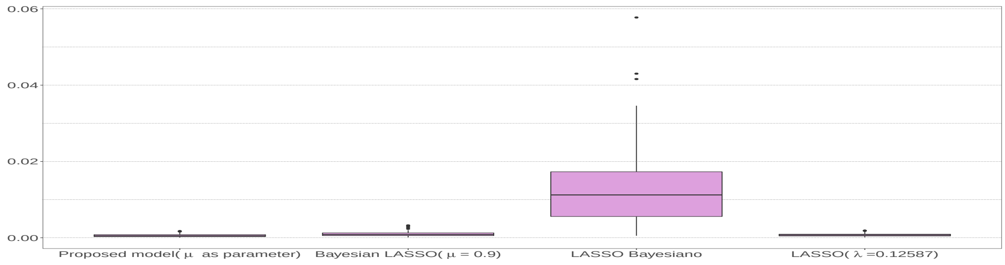


(a) Data with $\sigma = 0.1$.

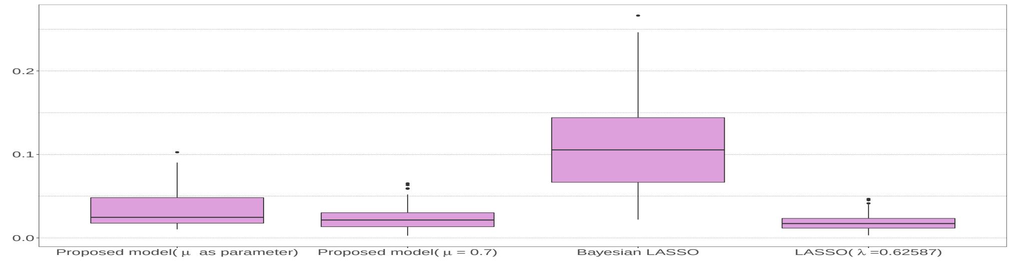


(b) Data with $\sigma = 0.5$.

Figure 4: Boxplots of the MSEs according to the model used and the data dispersion degree.

mance metric (16) was calculated for each value of $\lambda$ tested, and then the model with the $\lambda$ that returned the highest of these averages was selected for comparisons. Equivalently, the model with the value of $\mu$ which returned the highest average of the 100 values returned by the performance metric (16) was chosen for the comparison.

Regardless of the metric being analyzed, the superiority of the proposed model with $\mu$ as a parameter in relation to Bayesian LASSO is remarkable. This version of the proposed model that is compared with Bayesian LASSO has enough of a satisfactory performance to even be able to compete with LASSO, although a fairer comparison is restricted to evaluating LASSO against the proposed model with $\mu$ as the hyperparameter. In the latter case, it is also possible to note that both models have performances situated at the same level.

Next, Figures 5 and 6 present the boxplots of the final estimates from the respective coefficients defined for the versions of the proposed model, as well as the boxplots of the estimates from the coefficients that were defined by each adversary model chosen for comparison.

In analyzing the graphs, it is possible to conclude that Bayesian LASSO has a lower selection power when compared to the other models, while the proposed model accurately selects the base coefficients that were used in building the synthetic data, both in the version that competes with Bayesian LASSO, as well as in the version that competes with LASSO. The LASSO frequentist method is also able to accurately select the base coefficients, although it is not able to correctly select them with the same frequency as the proposed model. To reach such a conclusion, it is enough to note that the interquartile range of the boxplots associated with the coefficients that must be zeroed is greater in the estimates generated by LASSO. This happens for both data with $\sigma = 0.1$ and with $\sigma = 0.5$, but such difference is more noticeable in the latter case.

It is noteworthy that for $\sigma = 0.5$, the boxplots of final estimates 7 and 8 of the proposed

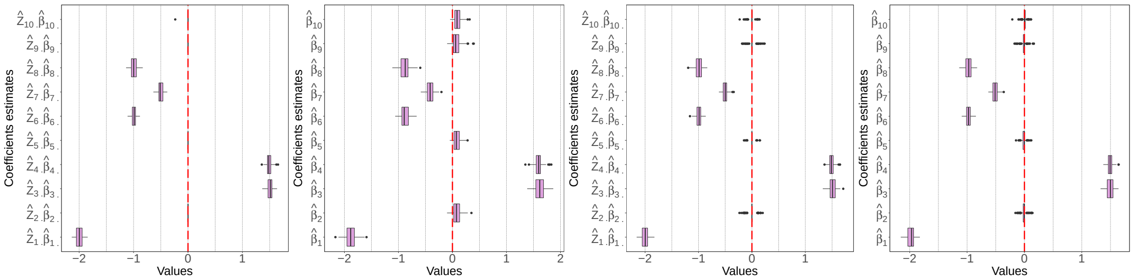


(a) Proposed model ($\mu$ as parameter). (b) Bayesian LASSO. (c) Proposed model with $\mu = 0.9$. (d) LASSO with $\lambda = 0.12587$.

Figure 5: Boxplots of the respective coefficient estimates for data with $\sigma = 0.1$, according to each model.

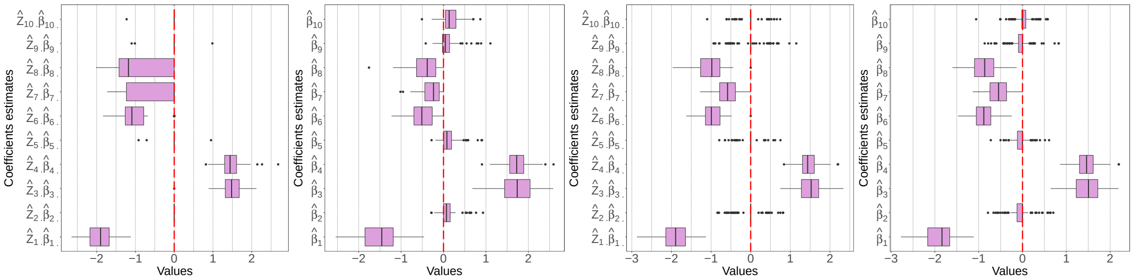


(a) Proposed model ($\mu$ as parameter). (b) Bayesian LASSO. (c) Proposed model with $\mu = 0.7$. (d) LASSO with $\lambda = 0.62587$.

Figure 6: Boxplots of the respective coefficient estimates for data with $\sigma = 0.5$, according to each model.

model which considers $\mu$ as a parameter (Figure 6a) have a larger interquartile range than the others, with the third quartile very close to zero, but even as such the coefficients are not zeroed.

For a brief analysis of the informativeness of the posterior values acquired by both the proposed model and by the Bayesian LASSO, the average value among the one hundred replications of the estimated variances of each coefficient was taken. For this situation, it is noteworthy that the partial coefficients ($\beta_k$s, without the subscript $i$ since $m = 1$) were used in the case of the proposed model versions.

Figure 7 shows the results obtained according to the data dispersion degree and model used.

As the data dispersion degree is small, Figure 7a is essential for understanding the proposed model's behavior in relation to the informativities of the posterior values. In this scenario, the proposed model for all coefficients that were selected, both with $\mu$ as a parameter and with $\mu$ fixed, returned more informative posterior values than the Bayesian LASSO. On the other hand, for all coefficients that were excluded from the proposed model, both with $\mu$ as a parameter and with $\mu$ fixed, the respective posterior values were extremely uninformative.

Although a similar pattern is observed when looking at Figure 7b, it can be seen that the two versions of the proposed model for the three coefficients which were defined closer to zero in the generation of the synthetic data return less informative posterior values than the Bayesian LASSO, suggesting that the closer to zero the coefficient is expected to be,

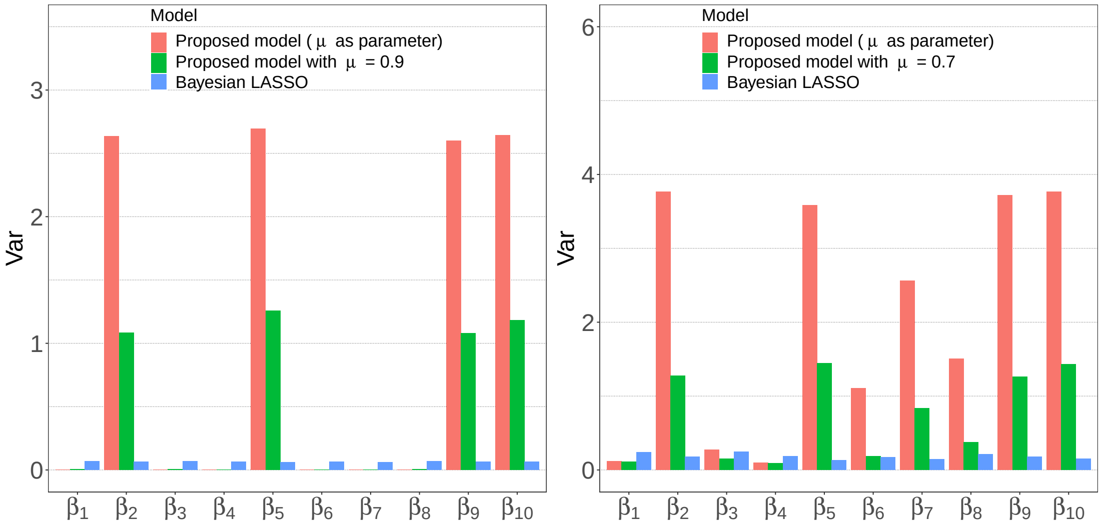


(a) $\sigma = 0.1$

(b) $\sigma = 0.5$

Figure 7: Average value of the estimated variances of each coefficient according to the data dispersion degree and the model used.

the less informative its respective posterior value should be. This behavior is evidently more easily observed when there is a greater data dispersion degree used.

A procedure often adopted as a final analysis to assess whether the Bayesian LASSO coefficients are truly null or not is characterized by the analysis of credibility intervals (CI). By constructing such intervals under a region whose density is maximum and considering a coverage fixed at a certain percentage, it is possible to calculate the proportions based on the total number of times among the one hundred replications that each coefficient estimate was different from zero.

Through these proportions, Figures 8 and 9 show the potential that each model has to identify the true bases, which were then used in the construction of the synthetic data.

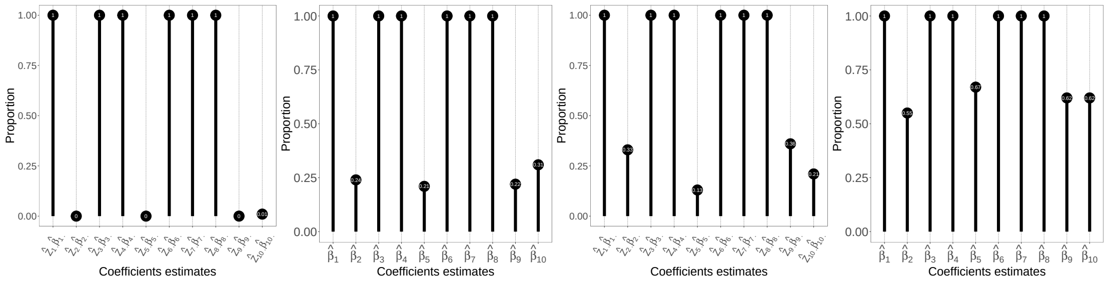


(a) Proposed model ($\mu$ as parameter).

(b) Bayesian LASSO with 50%CI of coverage.

(c) Proposed model with $\mu = 0.9$.

(d) LASSO with $\lambda = 0.12587$.

Figure 8: Proportions of non-zero estimates among the 100 replications for data with $\sigma = 0.1$, according to each model.

All models are able to clearly identify the bases that were used to generate the data for a low level of data dispersion, although the proportions of the bases that must be zeroed differ significantly among the models. The model proposed in its automated version, meaning

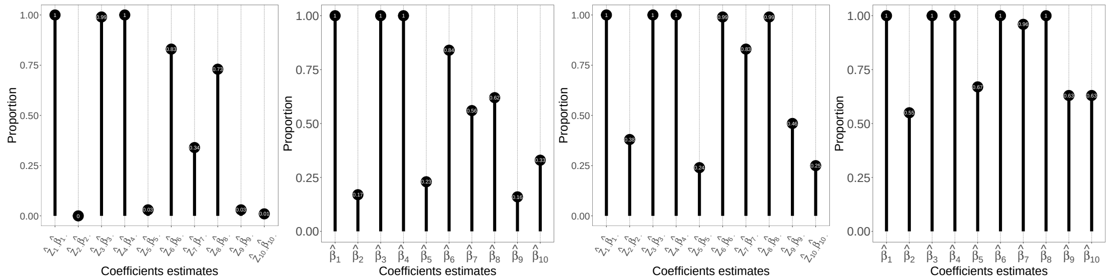


(a) Proposed model ($\mu$ as parameter). (b) Bayesian LASSO with 50%CI of coverage. (c) Proposed model with $\mu = 0.7$. (d) LASSO with $\lambda = 0.62587$.

Figure 9: Proportions of non-zero estimates among the 100 replications for data with $\sigma = 0.5$, according to each model.

with $\mu$ as a parameter, has the best results, since the proportions associated with the bases that must be excluded are almost all equal to zero. Then comes the proposed model with $\mu$ fixed at 0.7, which returns lower proportions for the coefficients that must be zeroed than those returned by LASSO. Finally, Bayesian LASSO has satisfactory results which are on the same level as the model in Figure 8c, but that loses in relation to its direct adversary, which is the model in Figure 8a.

A similar analysis can be attributed to the proportions presented for the data with a greater dispersion degree. However, it is noteworthy that the models in the latter case begin to show signs, even if small, of uncertainty in relation to the bases that should remain in the model.

This comparative analysis must be carried out with caution specifically for Bayesian LASSO, given the influence of the coverage percentage on the final value of the proportions. Figure 10 presents three graphs that result from different coverage percentages from the synthetic data generated with $\sigma = 0.1$. On the other hand, Figure 11 presents similar information from data with greater dispersion.

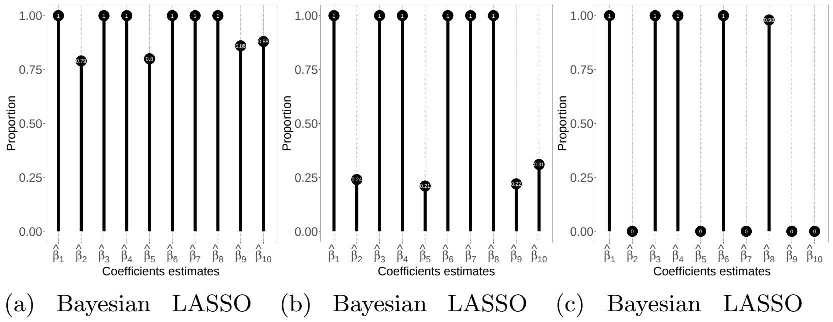


(a) Bayesian LASSO With 10%CI of coverage. (b) Bayesian LASSO with 50%CI of coverage. (c) Bayesian LASSO with 95%CI of coverage.

Figure 10: Proportions of non-zero estimates among the 100 replications for data with $\sigma = 0.1$, according to the percentage of coverage used.

The greater the coverage percentage of the coefficients' credibility intervals, evidently the greater the rigor for decision-making regarding which coefficients are different from zero.

When looking at Figures 10 and 11, it is noted that in the scenario with more intense regularization there is a greater discrepancy between the proportions associated with the

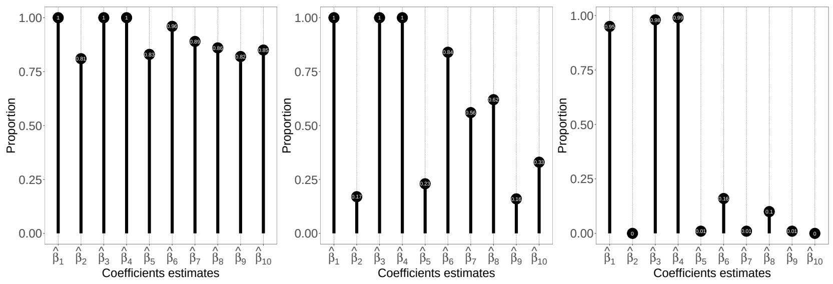


(a) Bayesian LASSO With 10%CI of coverage. (b) Bayesian LASSO with 50%CI of coverage. (c) Bayesian LASSO with 95%CI of coverage.

Figure 11: Proportions of non-zero estimates among the 100 replications for data with $\sigma = 0.5$, according to the percentage of coverage used.

coefficients that the model tends to select and those associated with the coefficients that the model tends to exclude. Although small proportions are indicative that the model has less uncertainty about the exclusion of the respective coefficient, it is worth noting that this does not necessarily indicate that the model is making the right decision. A good example is what happens with the seventh Bayesian LASSO coefficient with 95% coverage, which is associated with a proportion very close to zero, and it is a coefficient that should be selected.

In order to assess the quality of the Bayesian LASSO fit according to each of the percentages used to generate the graphs in Figures 10 and 11, all one hundred replications were taken for each fixed coverage percentage, and the estimated curves were calculated using exclusively the coefficients which are associated with a proportion greater than 0.5. In other words, the estimated curves were obtained without considering the coefficients whose proportions were smaller than 0.5.

With the curves estimated as described for each replication and each fixed coverage percentage, it becomes possible to construct different boxplots based on the metric (4), with the difference that the vector of coefficients will have components with null value whenever the respective coefficient is associated with a proportion smaller than 0.5.

Figure 12 shows the performance metric results for each tested configuration.

Based on a brief assessment of Figures 10 and 11, it appears that when considering a threshold of 0.5 in proportions as a criterion for deciding whether a given coefficient remains in the model or not, only the scenario which takes into account the CI with 50% coverage is able to exactly pinpoint which coefficients should be selected. Thus, the results observed in Figure 12 confirm what was expected, meaning that among the three percentages evaluated, the CI with 50% coverage enables better model performance.

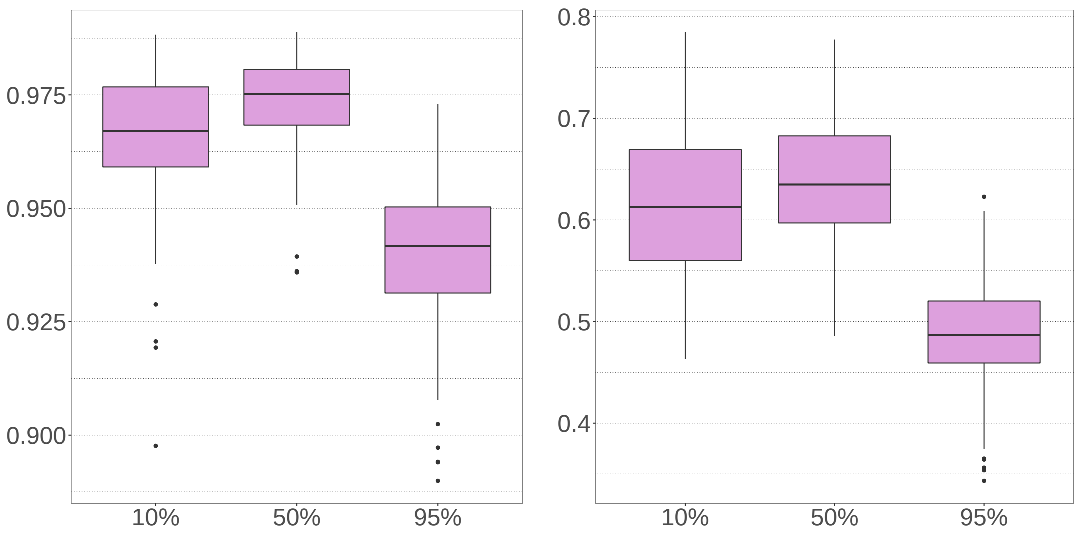


(a) $\sigma = 0.1$ (b) $\sigma = 0.5$

Figure 12: Metric (4) according to the coverage percentage and the data dispersion degree.

# A Boxplots for the Bayesian LASSO.

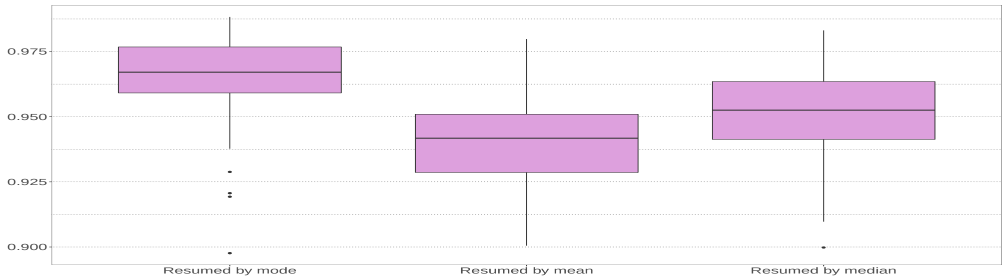


(a) Data with $\sigma = 0.1$

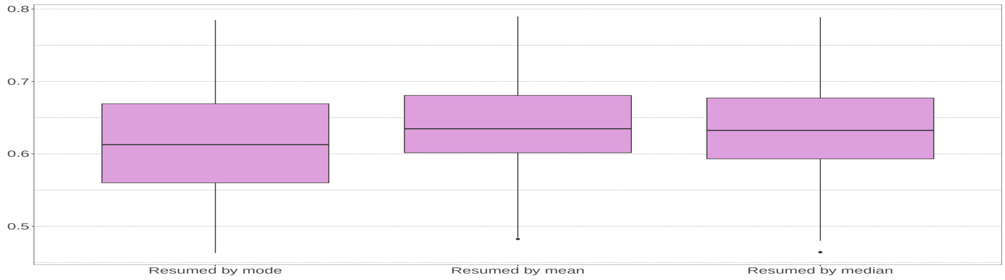


(b) Data with $\sigma = 0.5$

Figure 13: Boxplots of the metric (16) values from Bayesian LASSO according to the data dispersion degree and the posterior summary measure.

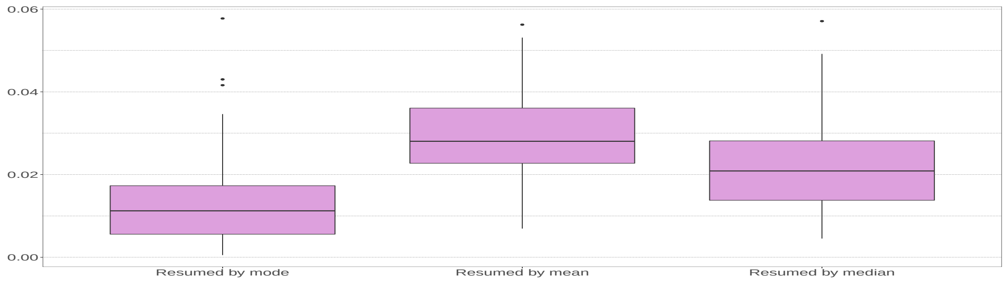


(a) Data with $\sigma = 0.1$

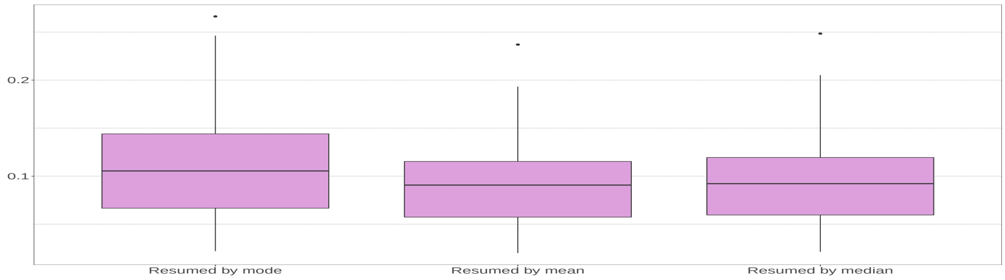


(b) Dada with $\sigma = 0.5$

Figure 14: Boxplots of MSE's from Bayesian LASSO according to the data dispersion degree and the posterior summary measure.

# B Sensibility by EQM of the models in relation to the regularization parameter.

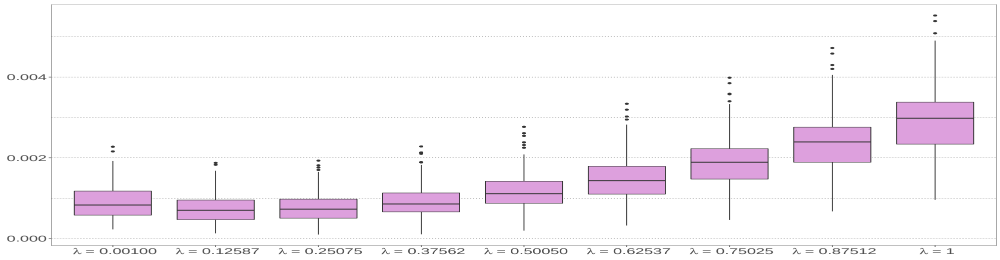


(a) Data with $\sigma = 0.1$.

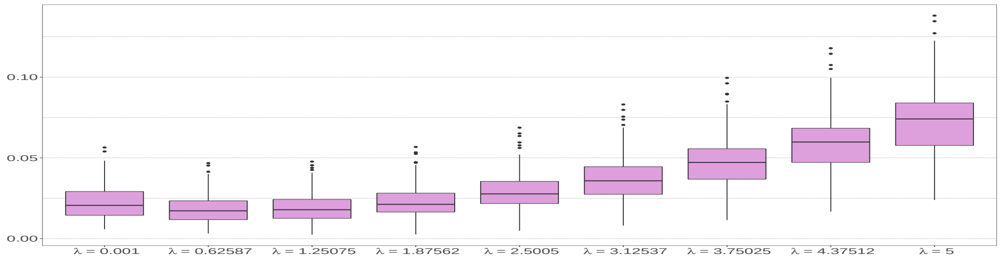


(b) Data with $\sigma = 0.5$.

Figure 15: Boxplots of the MSE's for the different LASSO model configurations tested, according to the data dispersion degree.

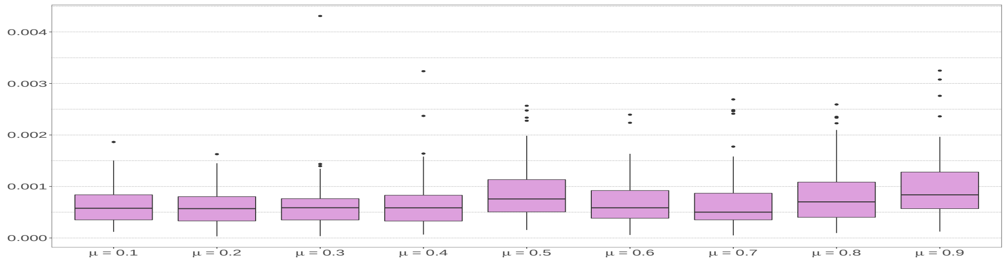


(a) Data with $\sigma = 0.1$.

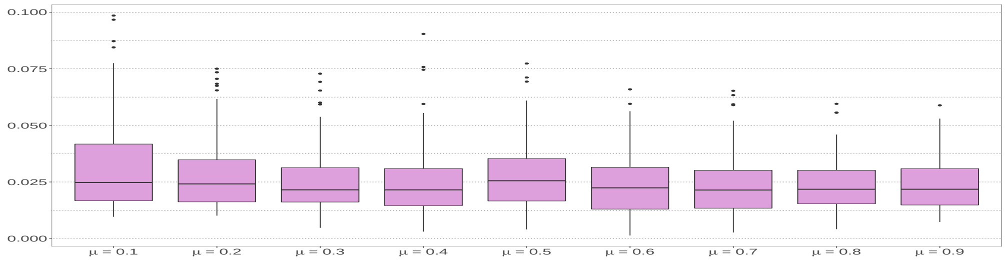


(b) Data with $\sigma = 0.5$.

Figure 16: Boxplots of the MSE's for the different proposed model configurations tested (with $\mu$ as hyperparameter), according to the data dispersion degree.

# References

Friedman, J., Hastie, T., and Tibshirani, R. (2010), "Regularization Paths for Generalized Linear Models via Coordinate Descent," *Journal of Statistical Software*, 33, 1–22.

Gramacy, R. B. (2018), *Estimation for Multivariate Normal and Student-t Data with Monotone Missingness*, CRAN, r package version 1.9.

Park, T. and Casella, G. (2008), "The Bayesian Lasso," *Journal of the American Statistical Association*, 103, 681–686.

Tibshirani, R. (1996), "Regression Shrinkage and Selection via the Lasso," *Journal of the Royal Statistical Society*, 58, 267–288.
